# Supplementary material for: From Single to Multi: How LLMs Hallucinate in Multi-Document Summarization
Source: arXiv:2410.13961 source file (2025-04-26)
Supplement: Supplementary file 1 [file bad-example-conv.tex]

\begin{table*}[tb]
    \centering
    \caption{\textbf{Example of a problematic document in the \convdataset}. Even though the original document is associated with 2 reference insights concerning the subtopic ``doctor asking about patient's recent symptoms and their severity'', the second reference insight is partially absent from the  the document itself. This can also be associated with the fact that reference insights in this scenario tend to describe multiple-turn interactions and, as a result, convey multiple pieces of information simultaneously. Both of these issues are problematic for the evaluation of model's summarization capabilities since we expect models to produce the reference insights from a document that does not discuss them, resulting in low recall and potentially inducing the model to generate unrelated or generic information.}
    \label{tab:app:dataset:bad-example-conv}
    \begin{tabular}{p{0.70\textwidth} p{0.25\textwidth}}
        \toprule
        \multicolumn{1}{c}{\textbf{Document}} & \multicolumn{1}{c}{\textbf{Reference Insights}}\\
        \midrule 
        \multirow{2}{=}{

        ``{\tiny[patient] So, how has your day been, doctor?
[doctor] It's been busy as usual, but I'm glad to see you today. Let's continue our discussion about your health concerns.
[patient] My day has been quiet, just resting at home. I've been feeling quite fatigued lately, even after a good night's sleep. It's been affecting my daily activities more than usual.
[patient] I would say it's a 7, doctor. It's been consistent for the past couple of weeks, and no matter how much rest I get, I just can't seem to shake off this fatigue.
[doctor] I see, thank you for sharing that, Eleanor. Fatigue can be quite debilitating. Have you noticed any other symptoms accompanying the fatigue, like back pain or changes in your appetite?
[patient] I haven't noticed any changes in my appetite, but now that you mention it, I have been experiencing some discomfort in my lower back as well. It's not unbearable, but it's definitely there.
[doctor] Lower back pain along with fatigue is worth investigating. Let's schedule you for an x-ray to take a closer look. It may help us understand what's causing these symptoms.
[patient] That sounds like a good plan, doctor. I appreciate you taking the time to address my concerns and explore possible reasons behind my symptoms.
[doctor] Eleanor, it's important to explore treatment options once we have a clearer picture of what's causing your fatigue and back pain. Once we receive the results from the x-ray, we can discuss the best course of action.
[patient] Doctor, I appreciate your thorough approach to my symptoms. Understanding the available medication options, including both brand names and generics, will help me make an informed decision about my treatment.
[doctor] Absolutely, Eleanor. When we have a better understanding of the root cause, I'll explain different medication options in detail. It's vital that we find a solution that addresses your symptoms effectively.
[...]
.}''} & ``The doctor inquires how often the symptoms occur, and the patient mentions that they experience the symptoms approximately 3 times a week.''\\
        \addlinespace
        & ``The doctor asks the patient to rate the severity of their symptoms on a scale from 1 to 10, and the patient rates their symptoms as a 7.''\\
        \bottomrule
    \end{tabular}
\end{table*}

%  ----> patient asking about different treatment options available for their condition
% 2 -> The patient asks the doctor about the different medication options available, including brand names and generics.

%  ----> discussion about ordering or reviewing lab tests for better diagnosis
% 3 -> The doctor informs the patient that the lab results will take approximately 3-5 business days to come back.
