# Supplementary material for: From Single to Multi: How LLMs Hallucinate in Multi-Document Summarization
Source: arXiv:2410.13961 source file (2025-04-26)
Supplement: Supplementary file 2 [file bad-example-news.tex]

\begin{table*}[tb]
    \small
    \centering
    \caption{\textbf{Example of a problematic document in the \newsdataset}. Even though the original document is associated with 4 reference insights concerning the subtopic ``Government measures and interventions taken to manage the crisis'', they are absent from the document itself. This reveals to be a problem for the evaluation of model's summarization capabilities since we expect models to produce the reference insights from a document that does not discuss them, resulting in low recall and potentially inducing the model to generate unrelated or generic information.}
    \label{tab:app:dataset:bad-example-news}
    \begin{tabular}{p{0.70\textwidth} p{0.25\textwidth}}
        \toprule
        \multicolumn{1}{c}{\textbf{Document}} & \multicolumn{1}{c}{\textbf{Reference Insights}}\\
        \midrule 
        \multirow{4}{=}{
        ``The sudden collapse of Silicon Valley Bank (SVB) has sent shockwaves throughout the financial sector, impacting a multitude of startups that relied heavily on its services. The history of Silicon Valley is filled with stories of innovation and collaboration. The economic landscape during such crises often brings to the forefront the collective efforts of various stakeholders, underpinned by community resilience. Throughout history, different financial sectors have responded to crises in unique ways. Founded in 1983 in Santa Clara, California, Silicon Valley Bank had long been a pillar of support for the tech industry. Over the years, it expanded its services to become a vital financial partner for thousands of startups. The region is a hub for talent and creativity, constantly pushing the boundaries of technology and business models. History has shown that during times of financial stress, innovative solutions often arise from collaborative efforts within the community. The community has historically come together in times of challenge to support one another. This reveals the vital importance of understanding how different financial ecosystems operate and adapt to crises. Silicon Valley Bank’s headquarters in Santa Clara is known for its iconic architectural design, symbolizing the bank's deep roots in the tech world. The early days of Silicon Valley saw rapid advancements and regulatory changes that helped shape the industry. Addressing these issues requires a balanced mix of strategic regulation and support to maintain stability. Prevailing financial conditions require carefully calibrated actions to ensure market stability and depositor confidence. Furthermore, understanding historical regulatory responses can provide valuable context. Government policies can significantly influence the outcome of financial crises. The collective intelligence and shared experiences are creating a new framework for dealing with financial crises. This model could serve as a blueprint for other sectors that might face similar challenges in the future. In summary, the fall of Silicon Valley Bank has led to a multifaceted response that combines governmental intervention with community-driven initiatives. From regulatory reforms to enhanced community resilience strategies, the response to this financial crisis has been robust and varied. The financial landscape is continuously evolving, requiring adaptive and dynamic responses from both the public and private sectors. Overall, this crisis has been a severe test of resilience for the startup community. However, the combined efforts of experienced entrepreneurs, community financial institutions, and a responsive government have provided a multifaceted safety net. This robust network of support might not only help these startups survive but could also solidify a new, more resilient financial frontier for future challenges. Visit telegraph.co.uk for more insights on this evolving story and detailed analyses of subsequent developments.''        
        } &  ``In response to the SVB collapse, central banks introduced emergency liquidity programs to ensure financial institutions could meet depositor needs and stabilize the market.''\\
        \addlinespace
        & ``Several of the nation's largest banks came together to inject \$30 billion into First Republic Bank, showcasing a coordinated effort to stabilize the banking sector.''\\
        \addlinespace
        & ``The bailout measures focused on protecting depositors, while shareholders and bondholders of SVB faced losses, thereby ensuring that the main victims were those who contributed to the risk.''\\
        \addlinespace
        & ``The federal government quickly announced that all deposits in Silicon Valley Bank would be guaranteed, aiming to quell panic and restore confidence in the banking system.'' \rule[-9em]{0pt}{0pt} \\

        \bottomrule
    \end{tabular}
\end{table*}

% other topic in this document...
%Community responses and grassroots efforts to support affected startups:
%  -> 4. Peer mentoring emerged as a critical component, with experienced entrepreneurs guiding those newer to the industry on navigating financial instability and exploring alternative funding routes.
%  -> 5. Liz Giorgi of soona emphasized the importance of direct advice among affected business owners, sharing that quick advice from peers on financial maneuvers has been crucial in mitigating immediate impacts.
%  -> 6. Community Development Financial Institutions (CDFIs) and credit unions have become crucial allies, offering tailored solutions for underserved communities and providing alternative banking options.
%  -> 7. Founders of affected startups have begun to collaborate to share resources and advice on finding new banking partners and securing credit lines. For instance, Vanessa Pham from Omsom noted that these collaborations were essential in securing a line of credit with JPMorgan Chase.
